# Supplementary material for: Versatile Reservoir Computing for Heterogeneous Complex Networks
Source: arXiv:2505.15219 source file (2025-05-21)
Supplement: Supplementary file 1 [file Supplementary.pdf]

Supplementary Material for

# **Versatile Reservoir Computing for Heterogeneous Complex Networks**

Yao Du, Huawei Fan, and Xingang Wang

Corresponding author: X. G. Wang (wangxg@snnu.edu.cn)

## **CONTENTS**

|                                                                                 |    |
|---------------------------------------------------------------------------------|----|
| I. Model A: homogeneous complex network of non-identical phase oscillators      | 2  |
| II. Model B: heterogeneous complex network of non-identical phase oscillators   | 4  |
| III. Model C: heterogeneous network of non-identical chaotic Lorenz oscillators | 5  |
| IV. Machine implementation details                                              | 6  |
| A. The general framework                                                        | 6  |
| B. Model A                                                                      | 8  |
| C. Model B                                                                      | 9  |
| D. Model C                                                                      | 9  |
| V. Factors influencing the machine performance                                  | 10 |
| References                                                                      | 12 |

## I. MODEL A: HOMOGENEOUS COMPLEX NETWORK OF NON-IDENTICAL PHASE OSCILLATORS

The network dynamics are governed by the set of equations

$$\dot{\theta}_i = \omega_i + \varepsilon \sum_{j=1}^N a_{ij} \sin(\theta_j - \theta_i), \quad (\text{S1.1})$$

where  $i, j = 1, \dots, N$  are the oscillator indices,  $\omega_i$  is the natural frequency of oscillator  $i$ ,  $\varepsilon$  denotes the uniform coupling strength, and  $\mathbf{A} = \{a_{ij}\}_{N \times N}$  is the adjacency matrix characterizing the coupling relationship of the oscillators. We have  $a_{ij} = a_{ji} = 1$  if there is a link between oscillators  $i$  and  $j$ , otherwise  $a_{ij} = 0$ . The natural frequencies  $\omega_i$  are independently sampled from a uniform distribution within the interval  $[-\pi/2, \pi/2]$ , and the initial phases of the oscillators are randomly chosen within the range  $(0, 2\pi]$ . The oscillators are of identical degree  $k = 3$ , and are connected at random in a frequency-assortative fashion (links are more likely to be established between oscillators with the similar natural frequencies) [1, 2]. Specifically, the probability of establishing a link between oscillators  $i$  and  $j$  is given by

$$p_{ij} \propto \frac{b^\gamma}{b^\gamma + |\omega_i - \omega_j|^\gamma}. \quad (\text{S1.2})$$

Following Ref. [1], here we set the parameters as  $b = 0.8$  and  $\gamma = 5$ . Compared to the conventional network models, chaotic dynamics can be observed in a wide regime in the parameter space of the frequency-assortative network model, making it a suitable model for evaluating the performance of the proposed machine-learning scheme. The network size is chosen as  $N = 50$ , and Eqs. (S1.1) is evolved numerically by the 4th-order Runge–Kutta algorithm with the time step  $\tau = 0.01$ .

The collective dynamics of the network are characterized by the synchronization order parameter

$$R(t) = \frac{1}{N} \left| \sum_{j=1}^N e^{i\theta_j(t)} \right|, \quad (\text{S1.3})$$

with  $\mathbf{i} = \sqrt{-1}$  being the imaginary unit and  $|\cdot|$  representing the modulus function. We have  $R(t) \in [0, 1]$ , with  $R(t) = 0$  and 1 corresponding to the completely desynchronized and globally synchronized states, respectively. The time-averaged synchronization order parameter,  $\langle R \rangle$ , is calculated over a time period of  $T = 1 \times 10^4$  (after discarding a transient period of  $T = 1 \times 10^2$ ).

Shown in Fig. S1(a) is the variation of the largest Lyapunov exponent,  $\Lambda$ , of the network dynamics with respect to the uniform coupling strength,  $\varepsilon$ . The variation of the time-averaged synchronization order parameter,  $\langle R \rangle$ , with respect to  $\varepsilon$  is plotted in Fig. S1(b). Dashed lines denote the sampling state,  $\varepsilon = 0.4$ , adopted in our studies for evaluating the effectiveness and efficiency of the proposed machine-learning scheme. The largest Lyapunov exponent of the sampling state is about  $\Lambda \approx 0.1$  (the corresponding Lyapunov time is about 10), and the time-averaged synchronization order parameter is about  $\langle R \rangle \approx 0.23$ .

In evaluating the performance of the machine in substituting a single oscillator in Model A (see Fig. 2 in the manuscript), it is found that the machine performance is dependent on the motion of the target oscillator (i.e., the oscillator that is substituted by the machine). Specifically, better performance is achieved when the target oscillator exhibits regular motion, and performance is worse

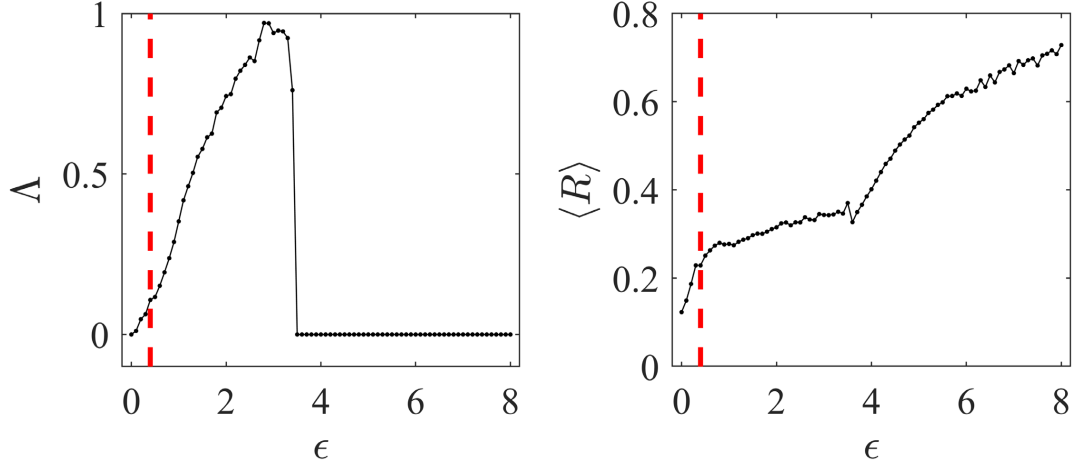

FIG. S1. For Model A (homogeneous complex network of non-identical phase oscillators), the variation of the largest Lyapunov exponent,  $\Delta$ , and the time-averaged synchronization order parameter,  $\langle R \rangle$ , with respect to the uniform coupling strength,  $\epsilon$ . Vertical dashed lines denote the sampling state adopted for evaluating the machine performance.

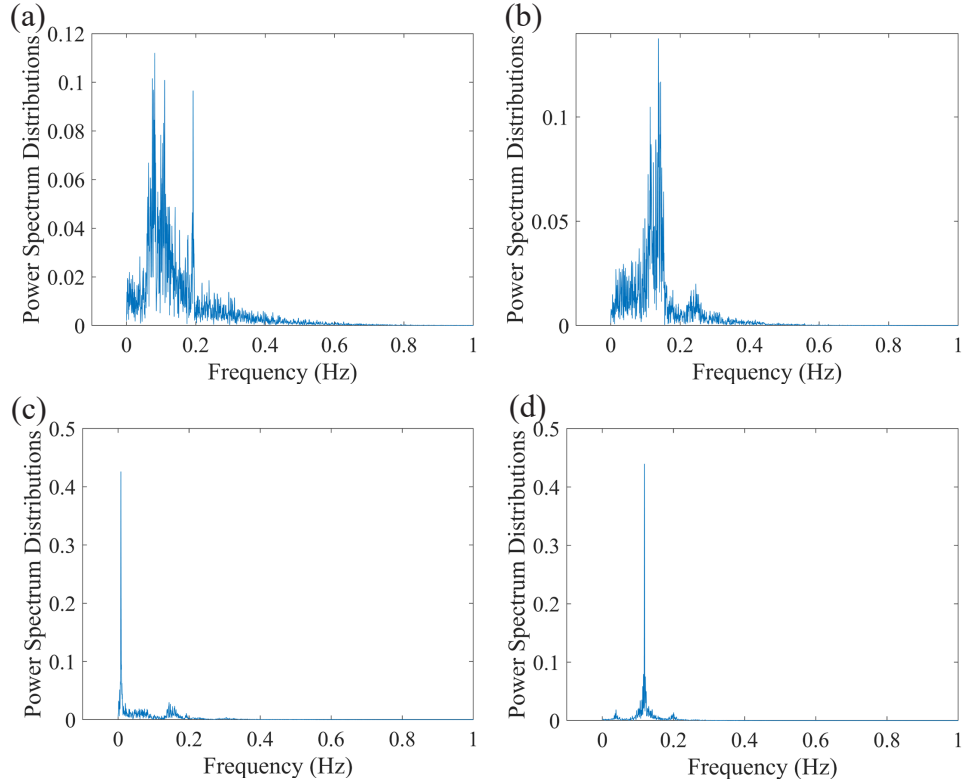

FIG. S2. For the sampling state depicted in Fig. S1 (Model A), the power spectrum distributions calculated from the time series of the oscillators studied in Figs. 2(a1-a4) in the manuscript. (a)  $\omega_{19} = 1.09$ . Irregular motion. (b)  $\omega_6 = -0.53$ . Irregular motion. (c)  $\omega_{45} = 0.21$ . Regular motion. (d)  $\omega_{26} = 0.30$ . Regular motion.

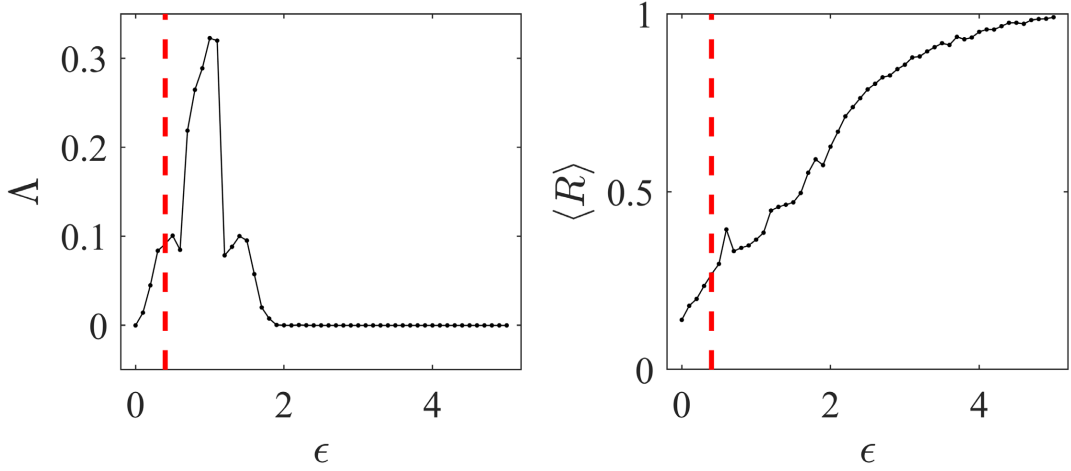

FIG. S3. For Model B (homogeneous complex network of non-identical phase oscillators), the variation of the largest Lyapunov exponent,  $\Lambda$ , and the time-averaged synchronization order parameter,  $\langle R \rangle$ , with respect to the uniform coupling strength,  $\varepsilon$ . Vertical dashed lines denote the sampling state adopted for evaluating the machine performance.

if the target oscillator displays irregular motion. To characterize the motions of the oscillators, we plot in Fig. S2 the distributions of the power spectrum for the oscillators studied in Figs. 2(a1-a4) in the manuscript. We see that the power spectrum distribution is broad in Figs. S2(a) and (b), indicating that the corresponding oscillators are of irregular motions. The narrow distributions presented in Figs. S2(c) and (d) suggest that the motions of the corresponding oscillators are highly regular.

## II. MODEL B: HETEROGENEOUS COMPLEX NETWORK OF NON-IDENTICAL PHASE OSCILLATORS

Except for the network structure, Model B is the same as Model A. In constructing the network of Model B, we first assign the oscillators with different degrees. The degrees are chosen randomly from the set  $k \in (2, 3, 4)$ . We then introduce links between paired oscillators by the probability described by Eq. (S1.2). The parameters defining the connecting probability are still chosen as  $(b, \gamma) = (0.8, 5)$ . Shown in Fig. S3(a) and (b) are the variation of the largest Lyapunov exponent,  $\Lambda$ , and the time-averaged synchronization parameter,  $\langle R \rangle$ , with respect to the uniform coupling strength,  $\varepsilon$ , for Model B. The sampling state adopted for evaluating the machine performance is chosen at  $\varepsilon = 0.4$ , for which we have  $\Lambda \approx 0.09$  and  $\langle R \rangle \approx 0.27$ .

To characterize the motions of the oscillators, we plot in Fig. S4 the power spectrum distributions for the same set of oscillators studied in Figs. 3(a1-a4) in the manuscript. We see that the distributions are broad in Figs. S4(a) and (b), indicating that the corresponding oscillators present irregular motions. The narrow distributions shown in Figs. S2(c) and (d) suggest that the motions of the corresponding oscillators are regular.

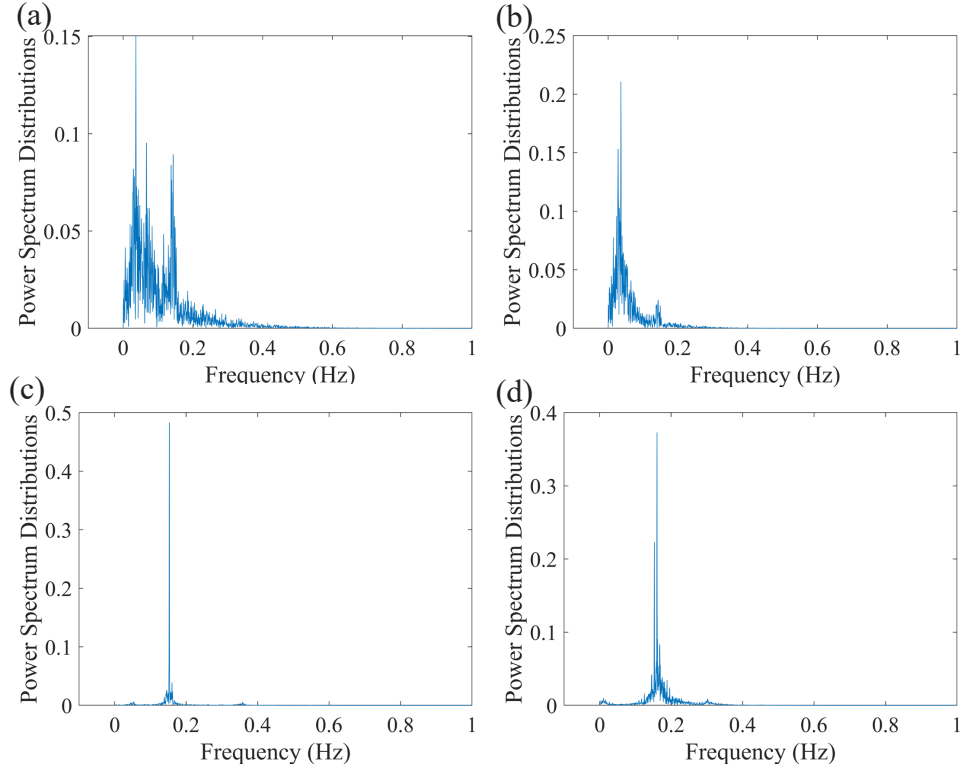

FIG. S4. For the sampling state depicted in Fig. S3 (Model B), the power spectrum distributions calculated from the time series of the oscillators studied in Figs. 3(a1-a4) in the manuscript. (a)  $\omega_1 = -0.20$ ,  $k = 4$ . Irregular motion. (b)  $\omega_{21} = 0.02$ ,  $k = 3$ . Irregular motion. (c)  $\omega_{24} = -1.27$ ,  $k = 2$ . Regular motion. (d)  $\omega_{22} = -1.37$ ,  $k = 2$ . Regular motion.

### III. MODEL C: HETEROGENEOUS NETWORK OF NON-IDENTICAL CHAOTIC LORENZ OSCILLATORS

Model C consists of  $N = 6$  oscillators and  $L = 7$  links, as depicted in Fig. S5. The degrees of the oscillators are  $(k_1, k_2, k_3, k_4, k_5, k_6) = (2, 3, 4, 2, 2, 1)$ . The network dynamics is governed by the set of equations

$$\begin{cases} \frac{dx_i}{dt} = 10(y_i - x_i) + \varepsilon_i \sum_{j=1}^N a_{ij}(x_j - x_i), \\ \frac{dy_i}{dt} = x_i(\beta_i - z_i) - y_i, \\ \frac{dz_i}{dt} = x_i y_i - 8/3 z_i, \end{cases} \quad (\text{S3.4})$$

with  $i, j = 1, \dots, 6$  the oscillator indices and  $\beta_i$  the intrinsic parameter characterizing the oscillator dynamics. The intrinsic parameters of the oscillators are chosen as  $(\beta_1, \beta_2, \beta_3, \beta_4, \beta_5, \beta_6) = (33.893, 33.332, 33.821, 33.042, 33.108, 33.595)$ . All oscillators present chaotic motions when isolated. In simulations, the initial states of the oscillators are randomly chosen within the range  $(0, 1)$ , and Eqs. (S3.4) are updated by the 4th-order Runge–Kutta algorithm with the time step  $\tau = 0.001$ . The coupling strength is set as  $\varepsilon = 0.5$ , with which the largest Lyapunov exponent of

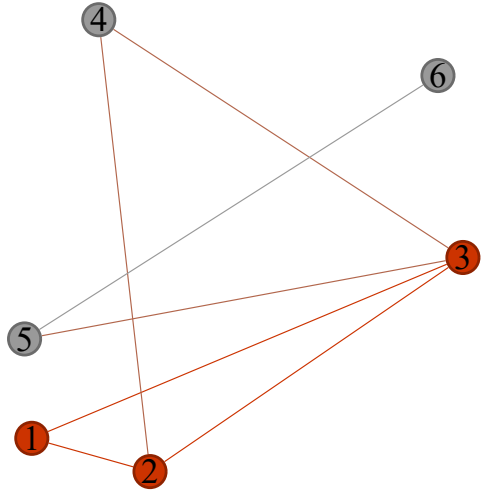

FIG. S5. The heterogeneous network consists of  $N = 6$  non-identical chaotic Lorenz oscillators. Sampled oscillators generating the training data are colored in red.

the network dynamics is about  $\Lambda = 1.1$  and the corresponding Lyapunov time is about 0.9.

#### IV. MACHINE IMPLEMENTATION DETAILS

##### A. The general framework

The technique of versatile reservoir computing (RC) proposed in the current study is generalized from the technique of parameter-aware RC proposed in Refs. [3, 4] by incorporating a coupling-signal channel into the input layer. Specifically, the machine is composed of three modules: the input layer, the hidden layer (reservoir network), and the output layer. The input layer is characterized by the matrix  $\mathbf{W}_{in} \in \mathbb{R}^{D_r \times D_{in}}$ , which couples the input vector  $\mathbf{U}(t) \in \mathbb{R}^{D_{in}}$  into the reservoir network. The input vector is expressed as  $\mathbf{U}_\beta(t) = [\mathbf{u}_\beta(t), \mathbf{u}_\beta^c(t), \beta(t)]^T$ . Here,  $\mathbf{u}_\beta(t) \in \mathbb{R}^{D_s}$  denotes the state vector of the target oscillator, which is inputted into the reservoir through the state channel;  $\mathbf{u}_\beta^c(t) \in \mathbb{R}^{D_c}$  represents the coupling vector the target oscillator receives from other oscillators in the system, which is inputted into the reservoir through the coupling channel;  $\beta(t)$  denotes the intrinsic parameter of the target oscillator, which is inputted through the parameter control channel. The elements of the input matrix,  $\mathbf{W}_{in}$ , are randomly drawn from a uniform distribution within the range  $[-\sigma, \sigma]$ . The reservoir network contains  $D_r$  nodes, with the initial states of the nodes being randomly chosen from the interval  $[-1, 1]$ . The states of the nodes in the reservoir network,  $\mathbf{r}(t) \in \mathbb{R}^{D_r}$ , are updated as

$$\mathbf{r}(t + \tau) = (1 - \alpha)\mathbf{r}(t) + \alpha \tanh[\mathbf{C}\mathbf{r}(t) + \mathbf{W}_{in}\mathbf{U}(t)]. \quad (\text{S4.5})$$

Here,  $\tau$  is the time step used for updating the reservoir network (for the sake of simplicity, we set it as the time interval of data sampling),  $\alpha \in (0, 1]$  is the leaking rate,  $\tanh$  represents the hyperbolic tangent function,  $\mathbf{C} \in \mathbb{R}^{D_r \times D_r}$  is a weighted adjacency matrix representing the coupling relationship between nodes in the reservoir network. The adjacency matrix  $\mathbf{C}$  is constructed as a sparse random Erdős-Rényi matrix: with the probability  $p$ , each element of the matrix is assigned a nonzero value drawn randomly from the interval  $[-1, 1]$ . The matrix  $\mathbf{C}$  is rescaled to make its spectral radius equal  $\lambda$ . The output layer is characterized by the matrix  $\mathbf{W}_{out} \in \mathbb{R}^{D_{out} \times D_r}$ , which generates the output vector,  $\mathbf{v}(t) \in \mathbb{R}^{D_{out}}$ , by the operation

$$\mathbf{v}(t + \tau) = \mathbf{W}_{out} \tilde{\mathbf{r}}(t + \tau), \quad (\text{S4.6})$$

where  $\tilde{\mathbf{r}}(t)$  is a modified state vector derived from the reservoir state vector  $\mathbf{r}(t)$ :  $\tilde{r}_i = r_i$  for odd-numbered nodes and  $\tilde{r}_i = r_i^2$  for even-numbered nodes. The output matrix,  $\mathbf{W}_{out}$ , is to be estimated from the measured data through a training process. Except  $\mathbf{W}_{out}$ , all other parameters of the machine, e.g.,  $\alpha$ ,  $\mathbf{W}_{in}$  and  $\mathbf{C}$ , are fixed at the construction.

As the standard RC, the implementation of the machine also contains three phases: training, validation, and application. The mission of the training phase is to find a suitable output matrix,  $\mathbf{W}_{out}$ , so that the output vector  $\mathbf{v}(t + \tau)$  as calculated by Eq. (S4.6) is as close as possible to the state vector  $\mathbf{u}_\beta(t + \tau)$  for  $t = \tau, \dots, L_t \tau$ , with  $L_t$  the length of the training series. This can be achieved by minimizing the cost function with respect to  $\mathbf{W}_{out}$ , which gives [5]

$$\mathbf{W}_{out} = \mathbf{M} \mathbf{V}^T (\mathbf{V} \mathbf{V}^T + \eta \mathbb{I})^{-1}, \quad (\text{S4.7})$$

where  $\mathbf{V} \in \mathbb{R}^{D_r \times L_t}$  is the state matrix whose  $k$ th column is  $\mathbf{r}(k\tau)$ ,  $\mathbf{M} \in \mathbb{R}^{D_{out} \times L_t}$  is a matrix whose  $k$ th column is  $\mathbf{u}_\beta(k\tau)$ ,  $\mathbb{I}$  is the identity matrix, and  $\eta$  is the ridge regression parameter for avoiding the overfitting. Please note that the state vector,  $\mathbf{u}$ , and the output vector,  $\mathbf{v}$ , are of the same dimension, i.e.  $D_{out} = D_s$ .

The machine that performs well on the training data might not perform equally well on the testing data. The finding of the optimal machine performing well on both the training and testing data is the mission for the validating phase. The set of hyperparameters to be optimized in the machine include  $D_r$  (the size of the reservoir network),  $p$  (the density of the adjacency matrix  $\mathbf{A}$ ),  $\sigma$  (the range defining the elements of the input matrix),  $\lambda$  (the spectral radius of the adjacency matrix  $\mathbf{A}$ ),  $\eta$  (the regression coefficient), and  $\alpha$  (the leaking rate). In our studies, the optimal hyperparameters are obtained by scanning each hyperparameter over a certain range in the parameter space using conventional optimization algorithms such as the Bayesian and surrogate optimization algorithms [3].

Having obtained the optimal machine, we then utilize it to substitute an oscillator randomly chosen in the system, namely the application phase. In doing this, we replace  $\mathbf{u}_\beta(t)$  with  $\mathbf{v}(t)$  (so that the machine is operating in the closed-loop mode), while setting  $\beta$  as the intrinsic parameter of the substituted oscillator. The machine is coupled with other oscillators in the system as the substituted oscillator. Specifically, the machine receives coupling signals,  $\mathbf{u}_\beta^c(t)$ , from other oscillators in exactly the same way as the oscillator that is substituted by the machine and, in the meantime, the output vector,  $\mathbf{v}(t)$ , is also coupled to the same set of neighbors as the substituted oscillator in the system. We note that the intrinsic parameters of the oscillators and the network structure are known *a priori*, yet the coupling functions and the oscillator dynamics are unknown.

## B. Model A

The instant phase of the  $i$ th oscillator is represented by the vector  $\mathbf{u}_i(t) = [\sin \theta_i(t), \cos \theta_i(t)]^T$ , and time series are acquired from  $m = 10$  oscillators sampled randomly in the network. For each sampled oscillator, a sequence of  $L = 5000$  data points is acquired by the time interval  $\tau = 10 \times \delta t = 0.1$ . Each sequence is split into two segments. The first segment contains  $L_t = 4000$  data points, which are used for training the output matrix. The second segment contains  $L_o = 1000$  data points, which are used for optimizing the machine hyperparameters. The training (validating) dataset is the concatenation of  $m$  time-series stacks,  $\tilde{\mathbf{U}} = (\mathbf{U}_1, \mathbf{U}_2, \dots, \mathbf{U}_m)$ , with  $\mathbf{U}_i \in \mathbb{R}^{D_{in} \times L_t}$  ( $\mathbb{R}^{D_{in} \times L_o}$ ) the input series associated with oscillator  $i$  within the sampling set. Data points in the  $i$ th stack is represented by the vector  $\mathbf{U}_i(t) = [\mathbf{u}_i(t), \mathbf{u}_i^c(t), \omega_i]^T$ , which has the dimension  $D_{in} = 2(k + 1) + 1$ , with  $k$  the uniform degree of the oscillators. As  $k = 3$  for Model A, we thus have  $D_{in} = 9$ . The coupling vector is expressed as  $\mathbf{u}_i^c(t) = \{\mathbf{u}_j(t)\}$ , with  $j$  the neighbors of oscillator  $i$  in the network. The state vector  $\mathbf{u}_i(t)$  is inputted into the reservoir through the state channel; the coupling vector  $\mathbf{u}_i^c(t)$  is inputted into the reservoir through the coupling channel; the natural frequency,  $\omega_i$ , is inputted into the reservoir through the parameter-control channel. Please note that the time series of the control parameter,  $\omega(t)$ , is a step-function in time [i.e.,  $\omega(t) \equiv \omega_i$  for  $\mathbf{U}_i$ ]. As  $m = 10$  oscillators are sampled, the length of the training and validating series are  $\tilde{L}_t = m \times L_t = 5 \times 10^5$  and  $\tilde{L}_o = m \times L_o = 1 \times 10^5$ , respectively.

The processes of machine training and optimization are the same as those of parameter-aware RC [3, 4], except that the input data includes the coupling signals,  $\mathbf{u}_i^c(t) \in \mathbb{R}^{2k}$ . Specifically, in the training phase, the input vector is  $\mathbf{U}_i(t)$ , and the cost function for estimating the output matrix is defined as the Euclidean distance ( $L^2$  norm) between the output vector  $\mathbf{v}(t + \tau)$  and the true state vector  $\mathbf{u}_i(t + \tau)$ . In this phase, the machine is operating in the open-loop mode. In the validation phase, we fix the reservoir size as  $D_r = 500$  for simplicity, while optimizing the other machine hyperparameters by minimizing the cost function over the validating dataset. The ranges over which the hyperparameters are tuned are  $[0, 1]$  for  $p$  (the density of the reservoir network),  $[0, 3]$  for  $\sigma$  (the range of the input matrix),  $[0, 3]$  for  $\lambda$  (the spectral radius of the reservoir),  $[1 \times 10^{-10}, 1 \times 10^{-2}]$  for  $\eta$  (the regression coefficient), and  $[0, 1]$  for  $\alpha$  (the leaking rate). In this phase, the machine is operating in the closed-loop mode by replacing  $\mathbf{u}_i(t)$  with  $\mathbf{v}(t)$  in the state channel (the inputs of the coupling and parameter-control channels are still from the validating data). The optimal hyperparameters are obtained after 300 trials searching in the parameter space with the help of the “optimoptions” function in MATLAB. The validation phase ends up with the set of optimal hyperparameters  $(p, \lambda, \sigma, \alpha, \eta) = (0.491, 0.090, 0.269, 0.365, 0.01)$ , which, together with the associated output matrix, defines the optimal machine to be used in the application phase.

In the application phase, the machine is first running in the open-loop mode by inputting a “warm-up” series (containing  $L_w = 50$  data points), and then operating in the closed-loop mode [depicted in Fig. 1(d1) in the manuscript] when it is used to substitute the target oscillator (which may or may not be included the sampling set). The “warm-up” series is acquired from the original system, whose function is to remove the impacts of the initial conditions of the reservoir. This process is carried out in an “offline” fashion (before substituting the target oscillator). After that, the machine is incorporated into the system as the digital twin of oscillator  $i$ . In doing this, the machine receives still coupling signals,  $\mathbf{u}_i^c(t)$ , from its neighbors in the system (through the coupling channel) and is also driven by the intrinsic parameter  $\omega_i$  (through the parameter-control channel), whereas  $\mathbf{u}_i(t)$  is replaced by the machine output  $\mathbf{v}(t)$  (in the state channel). From the output vector

$\mathbf{v} = (v_x, v_y)$ , we can estimate the instant phase of the machine,  $\theta_i(t) = \arctan(v_x/v_y) + \pi/2$  for  $v_x > 0$  and  $\theta_i(t) = \arctan(v - x/v - y) + 3\pi/2$  for  $v_x < 0$ , which is coupled to other oscillators in the system according to Eq. (S1.1). (When more than one oscillators are substituted, the same machine is deployed at different targets.)

### C. Model B

For Model B, the time series are still acquired from  $m = 10$  oscillators, which are chosen at random in the network. The sampled oscillators are of different degrees [as depicted in Fig. 1(a2) in the manuscript]: 8 oscillators with degree  $k = 2$ , 26 oscillators with degree  $k = 3$ , and 16 oscillators with degree  $k = 4$ . Padding technique is adopted to equalize the dimension of the input data acquired from different oscillators, with the details the following. Let  $k_{max}$  be the largest degree of the network and  $k_i$  be the degree of oscillator  $i$  (within the sampling set), we introduce  $k_v = k_{max} - k_i$  virtual oscillators as new neighbors of oscillator  $i$ . Let  $\mathcal{U}_j = \{\mathbf{u}_j(t)\}$  be the time series of a true neighbor of oscillator  $i$ , the virtual oscillators are created by delaying the time series with different constants:  $\mathcal{U}_l = \{\mathbf{u}_j(t - l\tau)\}$ , with  $l = 1, \dots, k_v$  the index of the virtual oscillators and  $\tau$  the time interval of data sampling. The oscillator  $j$  creating the virtual ones can be randomly chosen from the true neighbors, which does not affect the results. With the virtual oscillators, the oscillators are of identical degree ( $k_i = k_{max}$ ), and the uniform dimension of the input vector is  $D_{in} = 2 + 2k_{max} + 1$ . Taking oscillator 2 in Model B as an example, it is connected to oscillators 15 and 39 in the network, and has the degree  $k_2 = 2$ . As  $k_{max} = 4$ , we thus introduce  $k_v = k_{max} - k_2 = 2$  virtual oscillators as new neighbors of oscillator 2, as depicted in Fig. 1(c2) in the manuscript (the first motif). Here, we choose oscillator 39 (it could also be oscillator 15) as the neighbor that generates the virtual oscillators. As such, for the data acquired from oscillator 2, the corresponding input vector is  $\mathbf{U} = [\mathbf{u}_{15}(t), \mathbf{u}_{39}(t), \mathbf{u}_{39}(t - 2\tau), \mathbf{u}_{39}(t - \tau), \mathbf{u}_2(t), \omega_i]$ , which has the dimension  $D_{in} = 11$  (as  $\mathbf{u}_i \in \mathbb{R}^2$ ). The other settings of the training data are the same as those in Model A, including the sampling interval ( $\tau$ ) and the lengths ( $L_t$  and  $L_o$ ).

The training and validation procedures of the machine are the same as those of Model A. The optimal machine hyperparameters obtained through the “optimoptions” function in MATLAB are  $(p, \lambda, \sigma, \alpha, \eta) = (0.466, 0.151, 0.273, 0.38, 8 \times 10^{-3})$ . Still, the reservoir size is fixed as  $D_r = 500$  for simplicity. When it is used to substitute an oscillator in the network, the machine receives signals from both the true and virtual neighbors, but the machine output is only sent to the true ones. Except for this difference, the operation of the machine in the application phase is the same as that of Model A.

### D. Model C

For Model C, the training data are acquired from  $m = 3$  oscillators (as depicted in Fig. S5): one oscillator with degree  $k = 2$  (oscillator 1), one oscillator with degree  $k = 3$  (oscillator 2) and one oscillator with degree  $k = 4$  (oscillator 3). For each sampled oscillator, a sequence of  $L = 4000$  data points is acquired by the time interval  $\tau = 20 \times \delta t = 0.02$ . Data are normalized to be within the range  $[-1, 1]$ . Specifially, denoting  $v_{max}$  ( $v_{min}$ ) as the maximum (minimum) value of the variable  $v$  [with  $v \in (x, y, z)$ ] in the time series, the normalized variable is  $v' = 2(v - v_{min})/(v_{max} - v_{min}) - 1$ . [We can recover the variable  $v$  from the machine output  $v'$  by the

reverse operation:  $v = v_{min} + (v' + 1)(v_{max} - v_{min})/2$ .] Each sequence is split into two segments. The first segment contains  $L_t = 3000$  data points, which are used for training the output matrix. The second segment contains  $L_o = 1000$  data points, which are used for optimizing the machine hyperparameters. The state vector of oscillator  $i$  is  $\mathbf{u}_i' = [x_i', y_i', z_i']^T$ . The coupling signal that oscillator  $i$  receives from oscillator  $j$  is  $u_j = x_j - x_i$ . Again, padding technique is adopted to expand the dimension of the input vector. As  $k_{max} = 4$ , the uniform dimension of the input vector is  $D_{in} = 3 + 4 + 1 = 8$  (the additional dimension accounts for the intrinsic parameter,  $\beta$ , inputted into the reservoir through the parameter-control channel). The training and validation processes are the same as those of Models A and B. The reservoir size is fixed as  $D_r = 500$ , and the optimal hyperparameters of the machine are  $(p, \lambda, \sigma, \alpha, \eta) = (0.198, 0.233, 0.428, 0.195, 6 \times 10^{-3})$ . The operation of the machine in the application phase is the same as that of Model B.

## V. FACTORS INFLUENCING THE MACHINE PERFORMANCE

Besides the factors investigated in the manuscript (i.e., whether the substituted oscillator is included in the sampling set and whether the target oscillator has regular motion), the performance of versatile RC in sustaining the network dynamics is influenced by several other factors, including the number of the sampled oscillators on which the machine is trained, the number of oscillators that are substituted by the machine, and the uniform coupling strength. Additional simulations have been conducted to check the influences of these factors on the machine performance, and the general finding is that the machine performance will be improved when adopting more sampled oscillators or increasing the uniform coupling strength, but declines when more oscillators are substituted. In what follows, we take Model A as an example and demonstrate how the machine performance is affected by these additional factors.

The machine performance is improved with the number of sampled oscillators. Focusing on still the scenario of a single substitution (only one oscillator in the network is substituted by the machine), we plot in Fig. S6(a) the averaged maintenance horizon,  $\langle T_s \rangle$ , for machines trained on different number of oscillators,  $m \in (5, 10, 15, 20, 25)$ . For Models A and B, the maintenance horizon,  $T_s$ , is defined as the first time where the relative error,  $\delta E(t) = |R_o(t) - R_m(t)|/R_r(t)$ , exceeds the critical value 0.01, with  $R_o(t)$  and  $R_m(t)$  representing, respectively, the instant synchronization order parameters of the original network and the network with machine substitution. The value of  $\langle T_s \rangle$  is obtained by averaging  $T_s$  over all oscillators in the network ( $N = 50$  in total). We see in Fig. S6(a) (represented by the blue bars) that, with the increase of  $m$ , the value of  $\langle T_s \rangle$  is increased monotonically.

The machine performance is deteriorated when more oscillators are substituted. For the machine trained on  $m = 10$  oscillators in Model A (the same machine studied in Fig. 2 in the manuscript), the averaged maintenance horizon is about  $\langle T_s \rangle = 6.2$  Lyapunov times when it is deployed for substituting a single oscillator. When the same machine is deployed to substitute  $m_s = 2, 3$  and 4 oscillators, the averaged maintenance horizon is decreased to about  $\langle T_s \rangle = 5.1, 4$  and 3.8 Lyapunov times, respectively, as depicted in Fig. S6(a). In the scenario of multiple substitutions, the value of  $\langle T_s \rangle$  is averaged over 1000 realizations, while in each realization the substituted oscillators are chosen at random. Clearly, the performance of the machine in maintaining the network dynamics deteriorates gradually as more oscillators are substituted. The same trend is also observed for machines trained on different numbers of oscillators, as shown in Fig. S6(a).

The machine performance is improved with the increase of the uniform coupling strength,

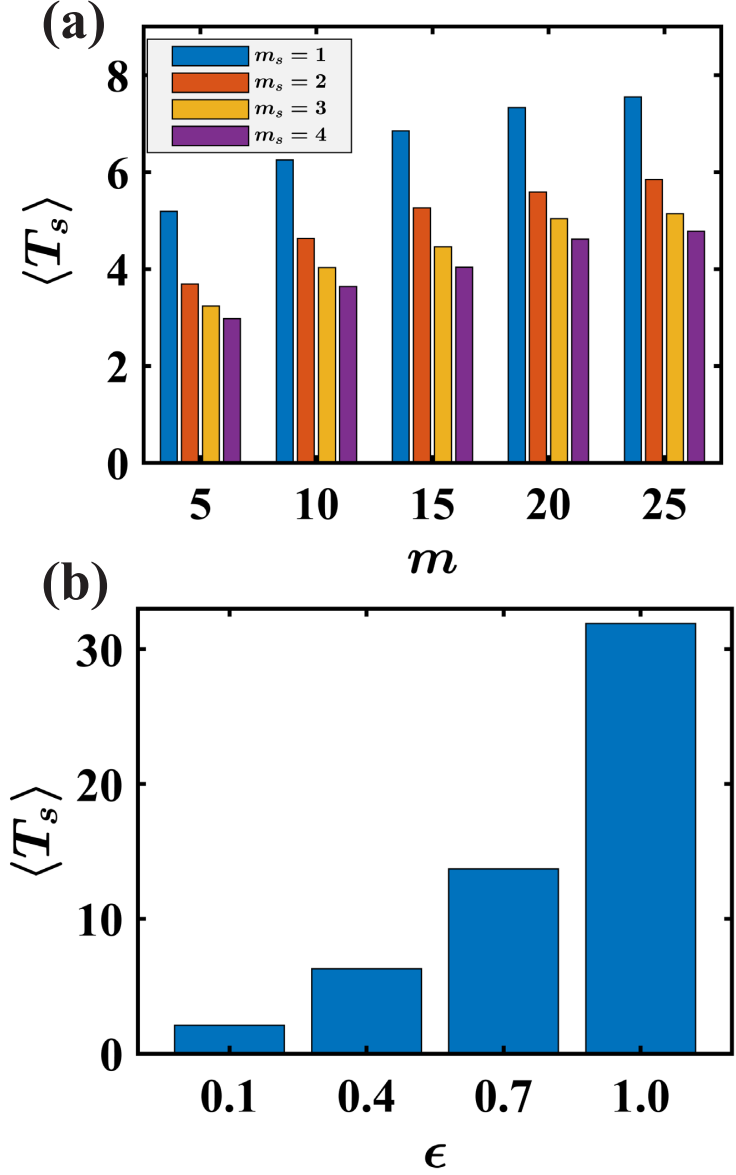

FIG. S6. For Model A, the factors that affect the machine performance. (a) The dependence of the averaged maintenance horizon,  $\langle T_s \rangle$ , on the number of sampled oscillators,  $m \in (5, 10, 15, 20, 25)$ , and the number of substitutions  $m_s \in (1, 2, 3, 4)$ . (b) The dependence of  $\langle T_s \rangle$  on the uniform coupling strength,  $\epsilon \in (0.1, 0.4, 0.7, 1.0)$ . Please see the context for details.

$\epsilon$ . With the other settings the same as those in Fig. 2 in the manuscript (the machine is trained on the time series of  $m = 10$  oscillators and a single oscillator is substituted by the machine), we plot in Fig. S6(b) the averaged maintenance horizon,  $\langle T_s \rangle$ , for different coupling strengths,  $\epsilon \in (0.1, 0.4, 0.7, 1.0)$ . The network dynamics is chaotic for all the coupling strengths, as depicted in Fig. S1(a). We see in Fig. S6(b) that  $\langle T_s \rangle$  is increased with  $\epsilon$  monotonically, suggesting that, compared with networks that are weakly synchronized, the strongly synchronized networks are more sustainable. This phenomenon is understandable, as the stronger the correlation among the

oscillators, the more similar the motions of the oscillators and, consequently, the more accurate the machine in replicating the oscillator dynamics.

---

- [1] J. G. Restrepo and E. Ott, Synchronization of oscillators: an ideal introduction to phase transitions, *EPL* **107**, 60006 (2014).
- [2] K. Srinivasan, N. Coble, J. Hamlin, T. Antonsen, E. Ott, and M. Girvan, Parallel machine learning for forecasting the dynamics of complex networks, *Phys. Rev. Lett.* **128**, 164101 (2022).
- [3] L.-W. Kong, H.-W. Fan, C. Grebogi, and Y.-C. Lai, Machine learning prediction of critical transition and system collapse, *Phys. Rev. Res.* **3**, 013090 (2021).
- [4] H. Fan, L.-W. Kong, Y.-C. Lai, and X. G. Wang, Anticipating synchronization with machine learning, *Phys. Rev. Res.* **3**, 023237 (2021).
- [5] J. Pathak, Z. Lu, B. Hunt, M. Girvan, and E. Ott, Using machine learning to replicate chaotic attractors and calculate Lyapunov exponents from data, *Chaos* **27**, 121102 (2017).
